# Supplementary material for: Free-Moving Object Reconstruction and Pose Estimation with Virtual Camera
Source: arXiv:2405.05858 source file (2024-05-10)
Supplement: Supplementary file 1 [file X_suppl.tex]

\clearpage
\setcounter{page}{1}
\maketitlesupplementary

% \section{Rationale}
% \label{sec:rationale}
% % 
% Having the supplementary compiled together with the main paper means that:
% % 
% \begin{itemize}
% \item The supplementary can back-reference sections of the main paper, for example, we can refer to \cref{sec:intro};
% \item The main paper can forward reference sub-sections within the supplementary explicitly (e.g. referring to a particular experiment); 
% \item When submitted to arXiv, the supplementary will already included at the end of the paper.
% \end{itemize}
% % 
% To split the supplementary pages from the main paper, you can use \href{https://support.apple.com/en-ca/guide/preview/prvw11793/mac#:~:text=Delete%20a%20page%20from%20a,or%20choose%20Edit%20%3E%20Delete).}{Preview (on macOS)}, \href{https://www.adobe.com/acrobat/how-to/delete-pages-from-pdf.html#:~:text=Choose%20%E2%80%9CTools%E2%80%9D%20%3E%20%E2%80%9COrganize,or%20pages%20from%20the%20file.}{Adobe Acrobat} (on all OSs), as well as \href{https://superuser.com/questions/517986/is-it-possible-to-delete-some-pages-of-a-pdf-document}{command line tools}.
\section{More Reconstruction Results}
\section{More Ablation Studies}

% \begin{table*}
%   \caption{\textbf{Comparison Among Multiple Camera Settings}(\textit{$ATE$ and $RPE_{t}$ use in the ratio of reconstructed object radius while $RPE_{r}$ is in degree, $AVG$ is average while $SD$ is standard deviation.}) \YH{Remove the 4D version (Change the 6D version to ``Virtual Camera Only'') and better to use separate groups for different metrics. }
%   }
%     \label{table:virtual_abalation}
%   \centering
%   \begin{tabular}{lccccccc}
%     \toprule
%     & \multicolumn{7}{c}{$ATE$/$RPE_{t}$/$RPE_{r}$} \\
%     Object &  Original & & 6 DoF Virtual && 4 DoF Virtual && Global Refine\\
%     \midrule
%     MC1 & 1.289/0.273/4.417 & & 0.309/0.120/2.072 & & 0.343/0.124/2.177 & & 0.218/0.098/1.645\\
%     ShSu12 & 0.544/0.157/2.760 & & 0.365/0.156/2.671  & & 0.321/0.146/2.521 & & 0.257/0.141/2.442\\
%     SM2 & 0.755/0.120/2.033 & & 0.757/0.124/1.996 & & 0.682/0.119/1.948 & & 0.661/0.105/1.723\\
%     ABF14 & 0.674/0.418/5.745 & & 0.456/0.199/3.381 & & 0.482/0.204/3.438 & & 0.462/0.142/2.551\\
%     MDF14 & 0.526/0.304/4.665 & & 0.212/0.073/1.321 & & 0.216/0.073/1.260 & & 0.148/0.069/1.228\\
%     AP13  &  0.208/0.060/1.163 & & 0.199/0.064/1.178 & & 0.192/0.069/1.260 & & 0.101/0.047/0.883\\
%     \midrule
%     $AVG$ & 0.666/0.222/3.464 & & 0.383/0.123/2.103 & & 0.373/0.122/2.101 & & \textbf{0.308/0.100/1.745}\\
%     $SD$  & 0.327/0.122/1.602 & & 0.189/0.046/0.757 & & \textbf{0.168}/0.046/0.754 & & 0.195/\textbf{0.035/0.599}\\
%   \bottomrule
%   \end{tabular}
% \end{table*}

% Move sequence-level numbers to supplementary
\begin{table*}%, $AVG$ is average while $SD$ is standard deviation.
  \caption{\textbf{Comparison Among Multiple Camera Settings}(\textit{$ATE$ and $RPE_{t}$ use in the ratio of reconstructed object radius while $RPE_{r}$ is in degree}) \YH{Remove the 4D version (Change the 6D version to ``Virtual Camera Only'') and better to use separate groups for different metrics. }
  }
    \label{table:virtual_abalation}
  \centering
  \begin{tabular}{l|ccc|ccc|ccc|ccc}
    \toprule
     \multirow{2}{*}{Object}&  \multicolumn{3}{c}{$AUC_{ATE}\uparrow$} & \multicolumn{3}{c}{$RPE_{t}\downarrow$} & \multicolumn{3}{c}{$RPE_{r}\downarrow$} & \multicolumn{3}{c}{$HD_{RMSE}\downarrow$}\\
     &  Orig. & 6 DoF & 4 DoF & Orig. & 6 DoF & 4 DoF & Orig. & 6 DoF & 4 DoF & Orig. & 6 DoF & 4 DoF\\
    \midrule

cracker box& 7.363& 7.428& \textbf{7.577}& 1.448& 1.705& \textbf{1.255}& 1.747& 2.041& \textbf{1.523}& 1.964& 1.771& \textbf{1.714}\\
sugar box& 6.777& \textbf{7.819}& 7.636& 1.824& \textbf{1.492}& 1.531& 2.851& \textbf{2.467}& 2.490& 2.655& 1.872& \textbf{1.837}\\
mustard bottle& 1.814& 3.920& \textbf{4.209}& 2.601& 1.161& \textbf{1.001}& 3.404& 1.695& \textbf{1.530}& 4.308& 3.579& \textbf{3.494}\\
bleach cleaner& 1.526& \textbf{5.311}& 5.307& 3.598& 1.956& \textbf{1.908}& 3.576& 2.721& \textbf{2.534}& 5.142& \textbf{4.911}& 5.379\\
potted meat& 1.674& 0.971& \textbf{3.061}& 5.482& 7.791& \textbf{1.921}& 8.792& 13.476& \textbf{2.906}& 3.760& 3.760& \textbf{1.803}\\
power drill& 4.095& 7.823& \textbf{8.537}& 5.731& 0.991& \textbf{0.977}& 7.240& 1.308& \textbf{1.278}& 5.069& 3.876& \textbf{3.824}\\
pitcher base& 7.416& \textbf{8.800}& 8.694& 0.923& \textbf{0.679}& 0.698& 1.127& \textbf{0.816}& 0.838& 6.279& \textbf{2.464}& 2.842\\
mug& 7.734& \textbf{8.217}& 8.095& 1.389& 1.079& \textbf{1.072}& 2.284& 1.758& \textbf{1.736}& 3.707& \textbf{2.674}& 2.777\\
banana& 0.539& \textbf{0.865}& 0.266& 14.223& \textbf{3.480}& 3.779& 33.671& 5.091& \textbf{4.959}& \textbf{4.488}& 4.538& 4.543\\

\midrule
Average&4.327&5.684&\textbf{5.931}&4.135&2.259&\textbf{1.571}&7.188&3.486&\textbf{2.199}&4.152&3.272&\textbf{3.135}\\

  \bottomrule
  \end{tabular}
\end{table*}

% Move sequence-level numbers to supplementary
\begin{table*}[tb!]
  \caption{\textbf{Abalation Study On Settings Of Segment-Free Progressive Training}(\textit{$ATE$ and $RPE_{t}$ use in the ratio of reconstructed object radius while $RPE_{r}$ is in degree, the metrics are in average for 7 objects in HO3D})
  }
  \centering
  \begin{tabular}{llcccc|ccccc|ccccc}
    \toprule
    \multirow{2}{*}{Setting} & \multirow{2}{*}{Metric}  & \multicolumn{4}{c}{Feeding Frame} & \multicolumn{5}{c}{Reset Degree} & \multicolumn{5}{c}{Match Interval}\\
    \multicolumn{2}{c}{} & 1 & 5 & 10 & 20 & 0 & 1 & 30 & 60 & 120 & 0 & 1 & 2 & 5 & 10\\
    \midrule

\multirow{4}{*}{virtual}& $AUC_{ATE}\uparrow$& \textbf{5.42}& 4.93& 5.14& 3.50& 5.15& 4.47& 5.34& 5.42& \textbf{5.48}& 4.91& 5.28& \textbf{5.65}& 5.53& 5.42\\
& $RPE_{t}\downarrow$& \textbf{1.94}& 2.18& 2.13& 2.42& \textbf{1.90}& 2.94& 2.18& 1.94& 1.96& 2.18& 2.21& 2.57& 2.08& \textbf{1.94}\\
& $RPE_{r}\downarrow$& \textbf{2.65}& 2.85& 2.80& 3.10& \textbf{2.60}& 3.58& 2.89& 2.65& 2.70& 2.72& 2.86& 3.15& 2.79& \textbf{2.65}\\
& $HD_{RMSE}\downarrow$& 3.90& 3.76& \textbf{3.76}& 4.40& 3.98& 4.42& 4.34& 3.90& \textbf{3.88}& 4.14& 4.20& 4.18& \textbf{3.80}& 3.90\\
 \midrule
\multirow{4}{*}{global}& $AUC_{ATE}\uparrow$& \textbf{5.93}& 5.43& 5.39& 3.76& 5.58& 5.05& 5.87& \textbf{5.93}& 5.68& 5.21& 5.68& 5.78& 5.81& \textbf{5.93}\\
& $RPE_{t}\downarrow$& \textbf{1.57}& 1.81& 1.79& 2.17& 1.64& 2.23& 1.71& \textbf{1.57}& 1.66& 1.87& 1.81& 2.19& 1.70& \textbf{1.57}\\
& $RPE_{r}\downarrow$& \textbf{2.20}& 2.41& 2.42& 2.76& 2.26& 2.83& 2.34& \textbf{2.20}& 2.37& 2.38& 2.44& 2.71& 2.35& \textbf{2.20}\\
& $HD_{RMSE}\downarrow$& \textbf{3.13}& 3.18& 3.15& 3.37& 3.28& 3.78& 3.52& \textbf{3.13}& 3.15& 4.10& 3.52& \textbf{3.01}& 3.06& 3.13\\
  \bottomrule
  \end{tabular}
  \label{table:ablation_study_seg}
\end{table*}

% Move sequence-level numbers to supplementary
\begin{table*}[tb!]
  \caption{\textbf{Abalation Study On Settings Of Segment-Free Progressive Training Per Object-1}(\textit{$ATE$ and $RPE_{t}$ use in the ratio of reconstructed object radius while $RPE_{r}$ is in degree})\HS{Likely this huge table will be put on supplementary materials}
  }
  \small
  \centering
  \begin{tabular}{llccccc|ccccc|ccccc}
    \toprule
    \multirow{2}{*}{Object} & \multirow{2}{*}{Setting} & \multirow{2}{*}{Metric}  & \multicolumn{4}{c}{Feeding Frame} & \multicolumn{5}{c}{Reset Degree} & \multicolumn{5}{c}{Match Interval}\\
    \multicolumn{3}{c}{} & 1 & 5 & 10 & 20 & 0 & 1 & 30 & 60 & 120 & 0 & 1 & 2 & 5 & 10\\
\midrule
\multirow{8}{*}{\shortstack{cracker \\ box}}& \multirow{4}{*}{virtual}& $AUC_{ATE}\uparrow$& 7.16& 6.87& 7.16& \textbf{7.51}& 6.85& 6.45& 6.94& 7.16& 7.17& 7.13& 7.02& 7.02& 7.06& 7.16\\
& & $RPE_{t}\downarrow$& 1.79& 1.84& \textbf{1.67}& 1.76& \textbf{1.61}& 2.27& 1.87& 1.79& 1.69& 1.77& \textbf{1.73}& 1.77& 1.78& 1.79\\
& & $RPE_{r}\downarrow$& 2.08& 2.21& \textbf{1.99}& 2.13& \textbf{1.90}& 2.64& 2.21& 2.08& 2.03& 2.10& \textbf{2.07}& 2.08& 2.07& 2.08\\
& & $HD_{RMSE}\downarrow$& 2.11& 2.14& \textbf{1.91}& 1.98& 2.20& 2.28& \textbf{2.03}& 2.11& 2.12& \textbf{2.08}& 2.32& 2.27& 2.31& 2.11\\
\cline{2-17}
& \multirow{4}{*}{global}& $AUC_{ATE}\uparrow$& 7.58& \textbf{7.59}& 7.49& 7.59& 7.01& 7.46& 7.60& 7.58& 7.59& 7.63& 7.59& 7.61& 7.55& 7.58\\
& & $RPE_{t}\downarrow$& 1.26& \textbf{1.21}& 1.23& 1.24& 1.38& 1.37& 1.28& 1.26& \textbf{1.22}& 1.26& 1.29& 1.29& \textbf{1.25}& 1.26\\
& & $RPE_{r}\downarrow$& 1.52& \textbf{1.47}& 1.50& 1.50& 1.65& 1.65& 1.52& 1.52& \textbf{1.50}& 1.53& 1.56& 1.57& 1.53& \textbf{1.52}\\
& & $HD_{RMSE}\downarrow$& 1.71& 1.76& \textbf{1.67}& 1.77& 1.86& 1.77& \textbf{1.71}& 1.71& 1.71& 1.99& 1.83& 1.77& 1.75& \textbf{1.71}\\
\midrule
\multirow{8}{*}{\shortstack{sugar \\ box}}& \multirow{4}{*}{virtual}& $AUC_{ATE}\uparrow$& 6.82& \textbf{6.91}& 6.79& 1.32& 6.66& 5.92& 6.77& 6.82& 7.31& 7.22& 7.21& 7.04& 7.01& 6.82\\
& & $RPE_{t}\downarrow$& \textbf{1.74}& 1.75& 1.75& 3.29& \textbf{1.59}& 1.93& 1.81& 1.74& 1.65& 1.72& \textbf{1.61}& 1.76& 1.72& 1.74\\
& & $RPE_{r}\downarrow$& \textbf{2.81}& 2.84& 2.86& 4.95& \textbf{2.65}& 3.18& 2.94& 2.81& 2.67& 2.87& \textbf{2.73}& 2.85& 2.82& 2.81\\
& & $HD_{RMSE}\downarrow$& 2.42& 2.39& \textbf{2.36}& 2.37& 2.62& \textbf{2.22}& 2.30& 2.42& 2.26& 2.31& 2.38& 2.45& \textbf{2.22}& 2.42\\
\cline{2-17}
& \multirow{4}{*}{global}& $AUC_{ATE}\uparrow$& \textbf{7.64}& 7.40& 7.34& 1.61& 7.51& 7.37& 7.57& 7.64& 7.95& 7.92& 7.91& 7.80& 7.70& 7.64\\
& & $RPE_{t}\downarrow$& 1.53& \textbf{1.53}& 1.54& 3.12& 1.51& 1.58& 1.62& 1.53& \textbf{1.49}& \textbf{1.52}& 1.53& 1.56& 1.53& 1.53\\
& & $RPE_{r}\downarrow$& \textbf{2.49}& 2.51& 2.51& 4.64& 2.47& 2.56& 2.61& 2.49& \textbf{2.45}& 2.50& 2.52& 2.53& \textbf{2.49}& 2.49\\
& & $HD_{RMSE}\downarrow$& \textbf{1.84}& 1.85& 1.97& 2.36& 2.15& 2.06& 1.95& \textbf{1.84}& 1.85& \textbf{1.78}& 1.99& 2.00& 1.94& 1.84\\
\midrule
\multirow{8}{*}{\shortstack{mustard \\ bottle}}& \multirow{4}{*}{virtual}& $AUC_{ATE}\uparrow$& \textbf{3.47}& 1.80& 1.70& 1.93& 3.50& 1.99& 2.40& 3.47& 4.15& 4.68& 4.97& 5.16& 4.02& 3.47\\
& & $RPE_{t}\downarrow$& 1.71& 1.80& 1.80& \textbf{1.69}& 1.79& 2.21& 2.04& 1.71& \textbf{1.63}& \textbf{1.59}& 1.98& 1.62& 1.83& 1.71\\
& & $RPE_{r}\downarrow$& \textbf{2.37}& 2.44& 2.47& 2.48& 2.47& 2.86& 2.68& 2.37& \textbf{2.31}& 2.29& 2.76& \textbf{2.27}& 2.52& 2.37\\
& & $HD_{RMSE}\downarrow$& 4.45& 4.29& \textbf{4.27}& 4.73& \textbf{4.11}& 4.37& 4.55& 4.45& 4.26& \textbf{4.18}& 4.30& 4.33& 4.35& 4.45\\
\cline{2-17}
& \multirow{4}{*}{global}& $AUC_{ATE}\uparrow$& \textbf{4.21}& 2.81& 1.61& 2.40& 3.94& 1.99& 2.30& 4.21& 3.66& 5.77& 4.85& 4.89& 3.68& 4.21\\
& & $RPE_{t}\downarrow$& \textbf{1.00}& 1.30& 1.45& 1.33& 1.22& 1.48& 1.24& \textbf{1.00}& 1.09& 1.10& 1.15& 1.01& 1.09& \textbf{1.00}\\
& & $RPE_{r}\downarrow$& \textbf{1.53}& 1.86& 1.95& 1.90& 1.80& 2.01& 1.75& \textbf{1.53}& 1.63& 1.73& 1.71& 1.53& 1.61& \textbf{1.53}\\
& & $HD_{RMSE}\downarrow$& 3.49& \textbf{3.47}& 4.20& 3.58& 3.53& 3.86& 3.73& \textbf{3.49}& 3.70& 4.06& 3.74& 3.77& 3.55& \textbf{3.49}\\
\midrule
\multirow{8}{*}{\shortstack{bleach \\ cleaner}}& \multirow{4}{*}{virtual}& $AUC_{ATE}\uparrow$& \textbf{5.25}& 1.73& 4.46& 2.25& 4.57& 3.00& 5.70& 5.25& 4.86& 3.03& 2.04& 5.31& 5.19& 5.25\\
& & $RPE_{t}\downarrow$& \textbf{2.22}& 3.06& 2.54& 3.49& \textbf{2.03}& 3.75& 2.24& 2.22& 2.26& 3.13& 3.01& 5.65& 2.22& \textbf{2.22}\\
& & $RPE_{r}\downarrow$& \textbf{2.80}& 3.38& 2.99& 3.32& \textbf{2.67}& 3.91& 2.85& 2.80& 2.84& 3.24& 3.63& 6.21& 2.83& \textbf{2.80}\\
& & $HD_{RMSE}\downarrow$& 5.31& 5.22& \textbf{5.20}& 5.40& \textbf{4.35}& 5.32& 5.30& 5.31& 5.15& \textbf{4.78}& 5.40& 5.12& 5.32& 5.31\\
\cline{2-17}
& \multirow{4}{*}{global}& $AUC_{ATE}\uparrow$& \textbf{5.31}& 1.96& 4.23& 2.48& 4.51& 3.33& 5.38& 5.31& 4.45& 2.99& 2.65& 3.79& 5.13& 5.31\\
& & $RPE_{t}\downarrow$& \textbf{1.91}& 2.77& 2.19& 3.20& \textbf{1.90}& 2.89& 1.99& 1.91& 2.05& 2.98& 2.55& 5.37& 2.00& \textbf{1.91}\\
& & $RPE_{r}\downarrow$& \textbf{2.53}& 3.25& 2.78& 3.16& 2.62& 3.30& 2.69& \textbf{2.53}& 2.78& 3.15& 3.31& 6.04& 2.68& \textbf{2.53}\\
& & $HD_{RMSE}\downarrow$& 5.38& 5.36& \textbf{4.80}& 5.40& 5.12& 5.05& \textbf{4.78}& 5.38& 5.03& 5.12& 4.99& 5.37& \textbf{4.94}& 5.38\\
\midrule
\multirow{8}{*}{\shortstack{potted \\ meat}}& \multirow{4}{*}{virtual}& $AUC_{ATE}\uparrow$& 2.49& \textbf{3.29}& 2.73& 0.87& 2.38& 1.97& 3.14& 2.49& 2.48& 3.23& 3.31& 3.03& 2.78& 2.49\\
& & $RPE_{t}\downarrow$& 2.45& 2.47& 2.80& \textbf{2.12}& \textbf{2.19}& 4.67& 2.72& 2.45& 2.20& 2.35& \textbf{2.29}& 2.34& 2.42& 2.45\\
& & $RPE_{r}\downarrow$& 3.67& 3.57& 4.27& \textbf{3.32}& 3.31& 6.64& 3.98& 3.67& \textbf{3.25}& 3.46& \textbf{3.37}& 3.49& 3.53& 3.67\\
& & $HD_{RMSE}\downarrow$& \textbf{1.94}& 1.99& 2.01& 1.99& \textbf{1.80}& 2.08& 2.05& 1.94& 1.83& 1.99& \textbf{1.93}& 1.98& 2.00& 1.94\\
\cline{2-17}
& \multirow{4}{*}{global}& $AUC_{ATE}\uparrow$& 3.06& \textbf{3.83}& 2.96& 0.84& 3.18& 2.41& 3.65& 3.06& 2.60& 3.14& 3.84& 3.20& 3.08& 3.06\\
& & $RPE_{t}\downarrow$& 1.92& 1.90& 2.41& \textbf{1.84}& \textbf{1.89}& 3.37& 1.96& 1.92& 1.90& 1.99& 1.90& 1.93& \textbf{1.85}& 1.92\\
& & $RPE_{r}\downarrow$& 2.91& \textbf{2.80}& 3.66& 2.85& \textbf{2.82}& 4.59& 2.90& 2.91& 2.83& 3.06& \textbf{2.78}& 2.85& 2.78& 2.91\\
& & $HD_{RMSE}\downarrow$& \textbf{1.80}& 1.92& 1.99& 1.96& 1.78& 1.96& 2.05& 1.80& \textbf{1.75}& 2.02& 1.69& 1.75& \textbf{1.67}& 1.80\\

  \bottomrule
  \end{tabular}
  \label{table:ablation_study_seg_per_obj_1}
\end{table*}

% Move sequence-level numbers to supplementary
\begin{table*}[tb!]
  \caption{\textbf{Abalation Study On Settings Of Segment-Free Progressive Training Per Object-2}(\textit{$ATE$ and $RPE_{t}$ use in the ratio of reconstructed object radius while $RPE_{r}$ is in degree})\HS{Likely this huge table will be put on supplementary materials}
  }
  \centering
  \small
  \begin{tabular}{lllcccc|ccccc|ccccc}
    \toprule
    \multirow{2}{*}{Object} & \multirow{2}{*}{Setting} & \multirow{2}{*}{Metric}  & \multicolumn{4}{c}{Feeding Frame} & \multicolumn{5}{c}{Reset Degree} & \multicolumn{5}{c}{Match Interval}\\
    \multicolumn{3}{c}{} & 1 & 5 & 10 & 20 & 0 & 1 & 30 & 60 & 120 & 0 & 1 & 2 & 5 & 10\\
\midrule
\multirow{8}{*}{\shortstack{power \\ drill}}& \multirow{4}{*}{virtual}& $AUC_{ATE}\uparrow$& 8.32& \textbf{8.35}& 7.82& 0.73& 7.69& 6.84& 7.90& 8.32& 8.09& 4.28& 6.75& 7.50& 8.11& 8.32\\
& & $RPE_{t}\downarrow$& 1.14& \textbf{0.97}& 1.13& 1.74& \textbf{1.12}& 1.49& 1.22& 1.14& 1.20& 1.30& 1.18& 1.24& 1.29& \textbf{1.14}\\
& & $RPE_{r}\downarrow$& 1.51& \textbf{1.32}& 1.53& 2.53& \textbf{1.49}& 1.78& 1.56& 1.51& 1.54& 1.72& 1.56& 1.62& 1.67& \textbf{1.51}\\
& & $HD_{RMSE}\downarrow$& \textbf{4.76}& 5.09& 5.19& 5.49& \textbf{4.62}& 5.38& 4.76& 4.76& 4.75& 4.39& 4.21& \textbf{4.10}& 4.73& 4.76\\
\cline{2-17}
& \multirow{4}{*}{global}& $AUC_{ATE}\uparrow$& 8.54& \textbf{8.54}& 8.35& 0.74& 7.74& 7.22& 8.49& 8.54& 8.26& 4.29& 6.90& 7.67& 8.22& 8.54\\
& & $RPE_{t}\downarrow$& 0.98& \textbf{0.93}& 0.96& 1.62& 1.01& 1.10& \textbf{0.96}& 0.98& 0.97& 1.09& 1.01& 1.01& 0.98& \textbf{0.98}\\
& & $RPE_{r}\downarrow$& 1.28& \textbf{1.24}& 1.28& 2.18& 1.29& 1.39& \textbf{1.25}& 1.28& 1.27& 1.41& 1.32& 1.31& 1.29& \textbf{1.28}\\
& & $HD_{RMSE}\downarrow$& 3.82& \textbf{3.31}& 3.46& 5.51& 3.23& 4.56& \textbf{2.99}& 3.82& 3.39& 4.01& 3.27& \textbf{2.63}& 3.44& 3.82\\
\midrule
\multirow{8}{*}{\shortstack{pitcher \\ base}}& \multirow{4}{*}{virtual}& $AUC_{ATE}\uparrow$& 7.39& 8.00& \textbf{8.18}& 8.17& 7.76& 7.56& 7.60& 7.39& 7.49& 7.32& 8.04& 7.99& 7.56& 7.39\\
& & $RPE_{t}\downarrow$& 1.01& 0.90& \textbf{0.84}& 0.91& 1.01& 1.27& 1.11& 1.01& \textbf{0.94}& 0.91& 0.89& \textbf{0.88}& 0.91& 1.01\\
& & $RPE_{r}\downarrow$& 1.13& 1.09& \textbf{0.99}& 1.04& 1.14& 1.49& 1.33& 1.13& \textbf{1.09}& 1.06& 1.07& 1.05& \textbf{1.05}& 1.13\\
& & $HD_{RMSE}\downarrow$& 5.88& 5.15& \textbf{4.73}& 5.40& 7.55& \textbf{5.58}& 5.63& 5.88& 6.46& \textbf{4.97}& 5.02& 5.21& 5.83& 5.88\\
\cline{2-17}
& \multirow{4}{*}{global}& $AUC_{ATE}\uparrow$& 8.69& 8.57& 8.55& \textbf{8.76}& 8.62& 8.67& 8.63& 8.69& 8.71& 7.26& 8.81& 8.84& 8.84& 8.69\\
& & $RPE_{t}\downarrow$& 0.70& 0.70& 0.70& \textbf{0.68}& 0.72& 0.73& 0.70& \textbf{0.70}& 0.70& 0.76& 0.71& 0.69& \textbf{0.67}& 0.70\\
& & $RPE_{r}\downarrow$& 0.84& 0.84& 0.84& \textbf{0.82}& 0.86& 0.87& 0.85& 0.84& \textbf{0.83}& 0.90& 0.85& 0.83& \textbf{0.81}& 0.84\\
& & $HD_{RMSE}\downarrow$& 2.84& 2.24& 2.55& \textbf{2.21}& 3.99& \textbf{2.30}& 2.55& 2.84& 3.22& 5.80& \textbf{2.14}& 2.15& 2.72& 2.84\\
\midrule
\multirow{8}{*}{\shortstack{mug}}& \multirow{4}{*}{virtual}& $AUC_{ATE}\uparrow$& \textbf{7.80}& 7.32& 7.01& 7.43& 6.86& 6.53& 7.50& 7.80& 7.73& 7.28& 7.72& 7.68& 7.79& 7.80\\
& & $RPE_{t}\downarrow$& \textbf{1.44}& 1.99& 1.52& 1.60& 1.53& 2.57& 1.90& 1.44& \textbf{1.39}& 1.49& \textbf{1.36}& 1.44& 1.41& 1.44\\
& & $RPE_{r}\downarrow$& \textbf{2.30}& 3.16& 2.49& 2.57& 2.43& 3.99& 2.95& 2.30& \textbf{2.23}& 2.43& \textbf{2.16}& 2.32& 2.29& 2.30\\
& & $HD_{RMSE}\downarrow$& 3.26& \textbf{3.10}& 3.17& 3.15& 4.00& 3.43& 3.35& \textbf{3.26}& 3.31& 3.51& 3.15& \textbf{3.03}& 3.16& 3.26\\
\cline{2-17}
& \multirow{4}{*}{global}& $AUC_{ATE}\uparrow$& 8.10& 7.84& 7.60& \textbf{8.19}& 7.53& 7.03& 8.03& 8.10& 7.87& 7.55& 7.92& 8.05& 7.98& 8.10\\
& & $RPE_{t}\downarrow$& \textbf{1.07}& 1.59& 1.17& 1.09& 1.21& 2.02& 1.52& \textbf{1.07}& 1.10& 1.21& 1.11& 1.11& 1.11& \textbf{1.07}\\
& & $RPE_{r}\downarrow$& \textbf{1.74}& 2.52& 1.88& 1.79& 1.94& 3.10& 2.38& \textbf{1.74}& 1.80& 1.95& 1.79& 1.80& 1.80& \textbf{1.74}\\
& & $HD_{RMSE}\downarrow$& \textbf{2.78}& 3.89& 3.23& 2.89& 3.30& 3.38& 2.85& \textbf{2.78}& 3.09& 2.99& 2.93& \textbf{2.71}& 2.97& 2.78\\
\midrule
\multirow{8}{*}{\shortstack{banana}}& \multirow{4}{*}{virtual}& $AUC_{ATE}\uparrow$& 0.13& 0.12& 0.42& \textbf{1.26}& 0.07& 0.00& 0.13& 0.13& 0.07& 0.05& 0.45& 0.16& 0.23& 0.13\\
& & $RPE_{t}\downarrow$& \textbf{3.98}& 4.85& 5.13& 5.22& 4.25& 6.31& 4.70& \textbf{3.98}& 4.64& 5.35& 5.79& 6.46& 5.11& \textbf{3.98}\\
& & $RPE_{r}\downarrow$& \textbf{5.15}& 5.61& 5.57& 5.59& 5.29& 5.73& 5.51& \textbf{5.15}& 6.39& 5.30& 6.38& 6.49& 6.32& \textbf{5.15}\\
& & $HD_{RMSE}\downarrow$& 4.97& \textbf{4.46}& 4.96& 9.10& \textbf{4.53}& 9.10& 9.10& 4.97& 4.83& 9.10& 9.10& 9.10& \textbf{4.30}& 4.97\\
\cline{2-17}
& \multirow{4}{*}{global}& $AUC_{ATE}\uparrow$& 0.27& 0.36& 0.36& \textbf{1.28}& 0.16& 0.00& 1.17& 0.27& 0.02& 0.31& 0.67& 0.14& 0.12& 0.27\\
& & $RPE_{t}\downarrow$& \textbf{3.78}& 4.35& 4.50& 5.40& 3.91& 5.54& 4.08& \textbf{3.78}& 4.44& 4.93& 5.08& 5.70& 4.81& \textbf{3.78}\\
& & $RPE_{r}\downarrow$& \textbf{4.96}& 5.24& 5.38& 5.98& \textbf{4.91}& 5.99& 5.14& 4.96& 6.27& 5.14& 6.14& 5.94& 6.14& \textbf{4.96}\\
& & $HD_{RMSE}\downarrow$& 4.54& 4.83& \textbf{4.52}& 4.65& 4.60& 9.10& 9.10& \textbf{4.54}& 4.61& 9.10& 9.10& 4.91& 4.56& \textbf{4.54}\\

  \bottomrule
  \end{tabular}
  \label{table:ablation_study_seg_per_obj-2}
\end{table*}
